# Supplementary material for: Imaging entanglement correlations with a single-photon avalanche diode camera
Source: arXiv:2001.03997 source file (2020-08-12)
Supplement: Supplementary file 1 [file SupplementaryInformation.pdf]

## I. DEPTH OF FOCUS ANALYSIS OF THE JOINT PROBABILITY DISTRIBUTION

Figure 1.a shows sum-coordinates images measured for different displacements $z$ of the crystal and the lens $f_1$ in the FF configuration. Similarly, Figure 1.b shows minus-coordinates images measured for different displacements $z$ of the crystal represented in the NF configuration. In both case, we observe a broadening of correlation with of photons pairs that is symmetric relative to the position in focus ($z = 0$). This effect is analogous to the diffraction of a focused Gaussian beam (first-order coherence) but transposed in the coincidence domain (second-order coherence). Using a double-Gaussian approximation for the two-photon wave-function, one can show that momentum and position correlation widths scale as $\sigma(z) = a\sqrt{1 + (bz/a^2)^{21}}$. By fitting the parameters $a$ and $b$, one can estimate the minimum correlation width $\sigma(0)$. The precision to which one can estimate the correlation width in this manner will naturally be affected by the pixel size of the camera: the larger the pixel, the less precise the estimation.

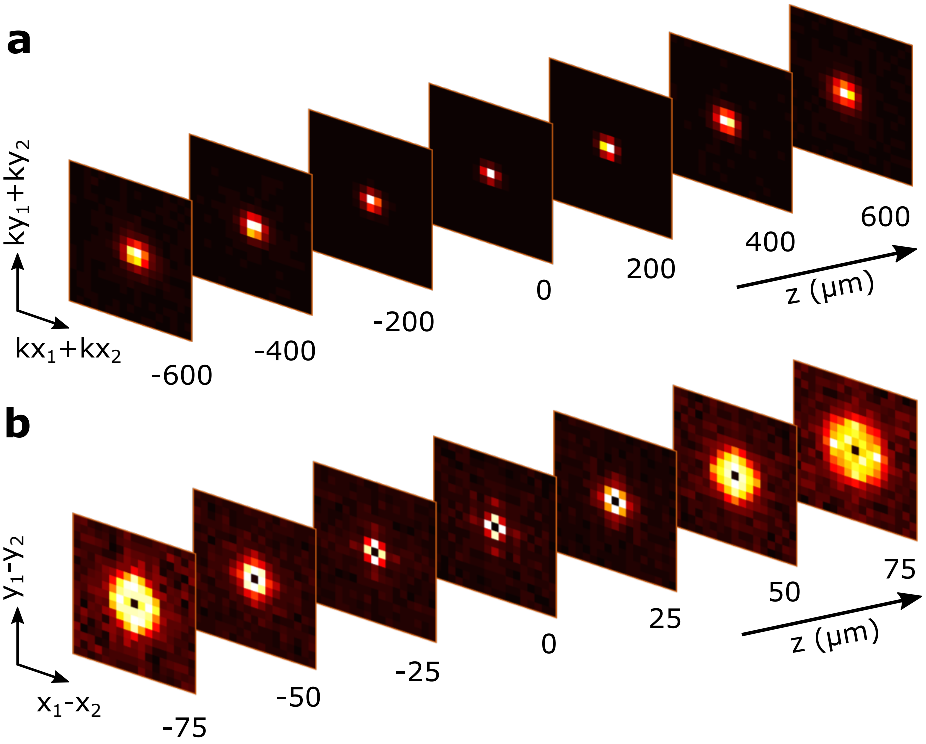


FIG. 1. **Depth of focus analysis.** **a**, Sum-coordinate projections of the JPD measured in the FF-configuration for different out-of-focus positions obtained by translating both the crystal and the lens $f_1$ by a displacement $z$ from the focal plane. **b,** Minus-coordinate projections of the JPD measured in the NF-configuration for different out-of-focus positions obtained by translating the crystal by a displacement $z$ from the focal plane.

## II. EFFECT OF PIXELATION ON THE GAUSSIAN FIT

As shown in Figures 2 and 3 of the manuscript, the correlation widths of the photon pairs produced by our source are on the order of the pixel size. This pixelation effect introduces uncertainties on the Gaussian fits and the extracted values of the correlation widths. Even if this error is difficult to quantify, it is important to note it can only lead to an overestimation of the correlation width values. Figure 2 shows simulations of the impact of this pixelation effect on the extracted correlation width values. First, we consider a theoretical Gaussian model of the form:

$$I_{th}(x) = e^{-\frac{x^2}{2\sigma_{th}^2}} \tag{1}$$

where $\sigma_{th}$ is a the theoretical width. We then generate pixelated data from this model by considering pixels of size 0.8 separated by a distance 0.2. These dimensions correspond to an imaging device with a fill fact of 80%, the same than the one of the SPAD camera used in our experiment. Blue crosses in Figures 2a and b show pixelated data

generated from Gaussian functions of widths $\sigma_{th} = 2$ and $\sigma_{th} = 0.1$, respectively. These pixelated data are then fitted by Gaussian models (red curves) that return width values of $\sigma_{fit} = 2.01$ and $\sigma_{fit} = 0.23$, respectively. As expected, these values are different from the theoretical ones because of the pixelation effect. However, it is essential to note that the values returned by the Gaussian fits are always larger than the theoretical values. This effect is confirmed in Figure 2.c that shows the extracted values $\sigma_{fit}$ in function of values of $\sigma_{th}$ ranging from 0.05 to 2 (i.e. the red curve is above the black dashed unity slope curve). In particular, when the theoretical width is much smaller than the pixel size, the value returned by the fit is approximately constant and equal to 0.2. This simulations show that the pixelation effect can only lead to an overestimation of the real Gaussian width values.

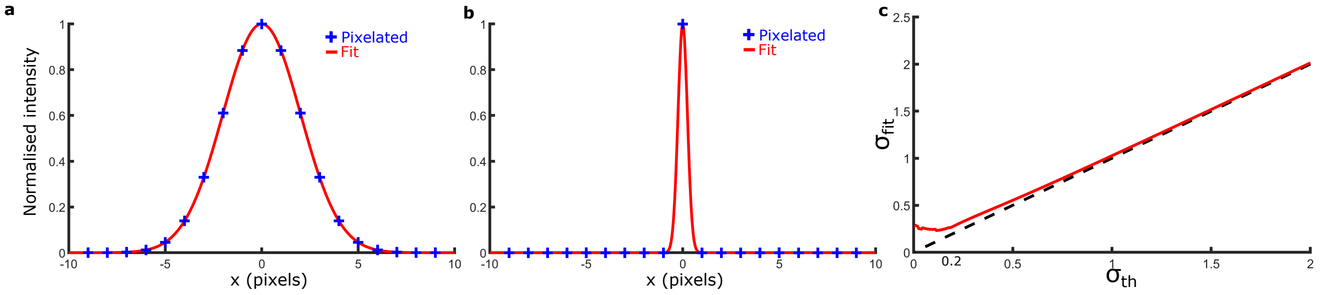


FIG. 2. **Pixelation effect.** **a**, Pixelated data produced by a Gaussian function of width $\sigma_{th} = 2$ (blue crosses) and Gaussian fit that returns a width of $\sigma_{fit} = 2.01$ (red curve). **b**, Pixelated data produced by a Gaussian function of width $\sigma_{th} = 0.1$ (blue crosses) and Gaussian fit that returns a width of $\sigma_{fit} = 0.24$ (red curve). **c**, Values of $\sigma_{fit}$ returned by the Gaussian fit in function of the theoretical values $\sigma_{th}$. Black dashed line is a linear curve with a slope of 1.

[1] M. Reichert, X. Sun, and J. W. Fleischer, Physical Review A **95**, 063836 (2017) .
